# Supplementary material for: Robust large-gap topological insulator phase in transition-metal chalcogenide ZrTe$_4$Se
Source: arXiv:2106.04035 source file (2021-06-08)
Supplement: Supplementary file 1 [file supplemental_material.pdf]

**SUPPLEMENTAL MATERIAL**

# Robust large-gap topological insulator phase in transition-metal chalcogenide $ZrTe_4Se$

Xing Wang,[1,2] Wenhui Wan,[1] Yanfeng Ge,[1] and Yong Liu[1,*]

[1]*State Key Laboratory of Metastable Materials Science and Technology & Key Laboratory for Microstructural Material Physics of Hebei Province, School of Science, Yanshan University, Qinhuangdao 066004, China*

[2]*College of Science, Hebei North University, Zhangjiakou 07500, China*

(Dated: June 8, 2021)

This Supplemental Material is meant to support the explanations described in the main text entitled “Robust large-gap topological insulator phase in transition-metal chalcogenide $ZrTe_4Se$”.

Part I The band struture of single-layer $ZrTe_4Se$ without considering the spin-orbit coupling by using the hybrid functional HSE06.

Part II The formula for binding energy and formation energy of $ZrTe_4Se$.

Part III The total potential energy fluctuation by using ab initio Molecular Dynamics (MD) simulation for $ZrTe_4Se$.

Part IV The snapshots of atomic configurations at the end of MD simulation for bulk $ZrTe_4Se$.

Part V The snapshots of atomic configurations at the end of MD simulation for single-layer $ZrTe_4Se$.

Part VI The evolution lines of Wannier centers for single-layer $ZrTe_4Se$.

Part VII The total potential energy fluctuation by using ab initio MD simulation for bulk $ZrTe_4Se$ certain strain.

Part VIII The evolution lines of Wannier centers for bulk $ZrTe_4Se$ under 3 % uniaxial strain.

Part I The band struture of single-layer $ZrTe_4Se$ without considering the spin-orbit coupling by using the hybrid functional HSE06.

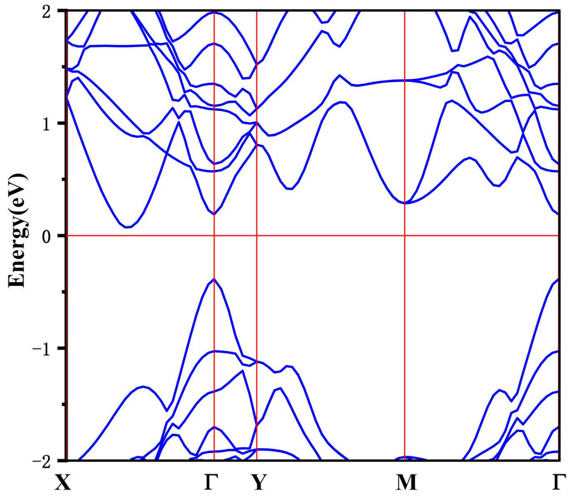


FIG. S1. (Color online) The band struture of single-layer $ZrTe_4Se$ without considering the spin-orbit coupling by using the hybrid functional HSE06.

Part II The formula for binding energy and formation energy of $ZrTe_4Se$.

The binding energy $E_b$, defined as

$$E_b = \frac{E(ZrTe_4Se) - 2E(Se) - 8E(Te) - 2E(Zr)}{12}, \tag{1}$$

where $E(ZrTe_4Se)$, E(Te), E(Se) and E($Zr$) are the energy of single-layer $ZrTe_4Se$, Te atom, Se atom and Zr atom respectively.

The formation energy $E_f$ is defined as

$$E_f = \frac{E_{2D}}{N_{2D}} - \frac{E_{3D}}{N_{3D}}, \tag{2}$$

where $E_{2D}$ ($E_{3D}$) and $N_{2D}$ ($N_{3D}$) are ground state energy and number of atoms of singer-layer (bulk) crystal respectively.

Part III The total potential energy fluctuation by using ab initio MD simulation for $ZrTe_4Se$.

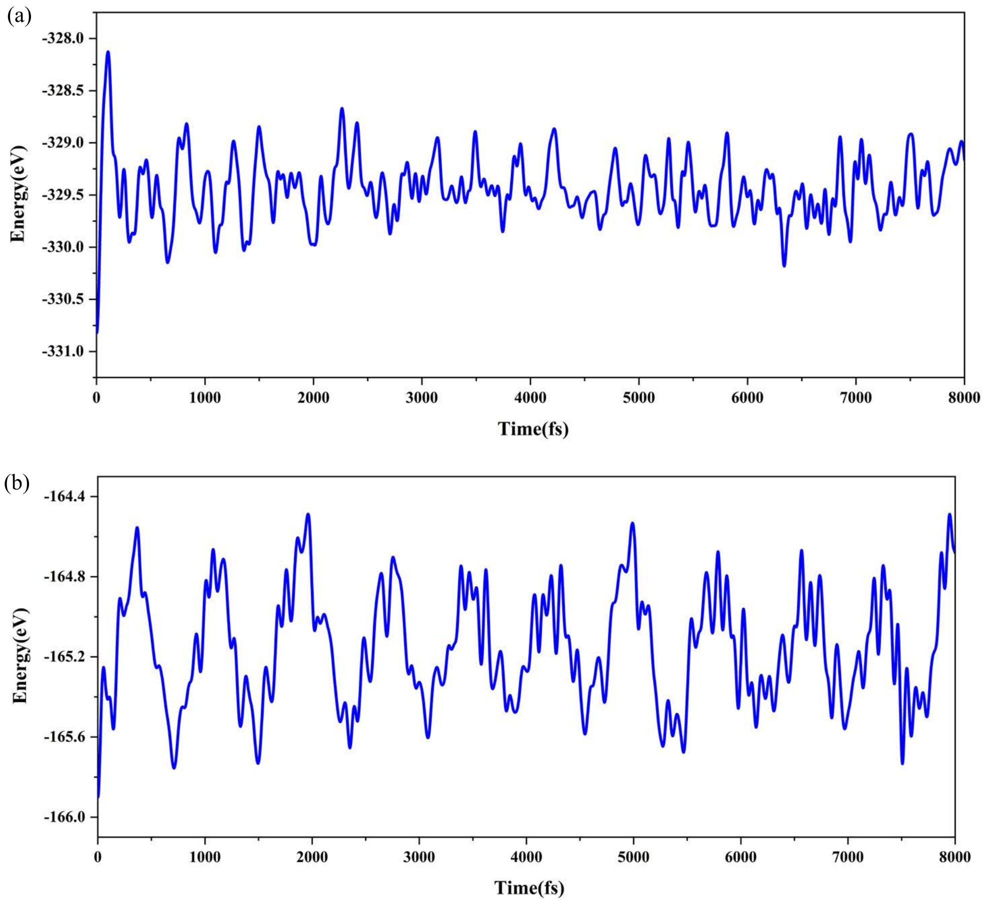


FIG. S2. (Color online) The total potential energy fluctuation during MD simulation at 300 K for (a) bulk and (b) single-layer of $ZrTe_4Se$.

Part IV The snapshots of atomic configurations at the end of MD simulation for bulk $ZrTe_4Se$.

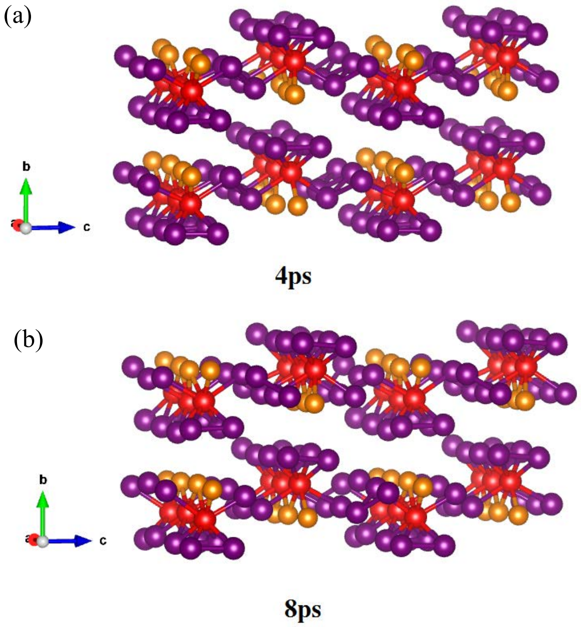


FIG. S3. Snapshots of atomic configurations at the end of MD simulation for (a) 4ps and (b) 8ps for single-layer of $ZrTe_4Se$.

Part V The snapshots of atomic configurations at the end of MD simulation for single-layer $ZrTe_4Se$.

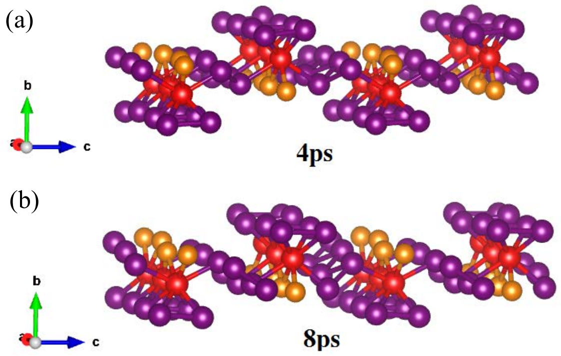


FIG. S4. Snapshots of atomic configurations at the end of MD simulation for (a) 4ps and (b) 8ps for single-layer of $ZrTe_4Se$.

Part VI The evolution lines of Wannier centers for single-layer $ZrTe_4Se$.

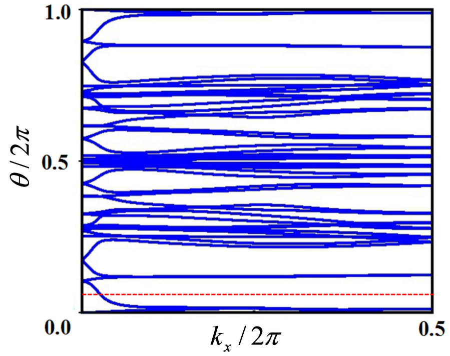


FIG. S5. The evolution of Wannier charge centers of single-layer $ZrTe_4Se$. The evolution of Wannier charge centers along $k_x$, the evolution blue lines cross the arbitrary reference red line one time yielding $Z_2$=1.

Part VII The total potential energy fluctuation by using ab initio MD simulation for bulk $ZrTe_4Se$ under certain strain.

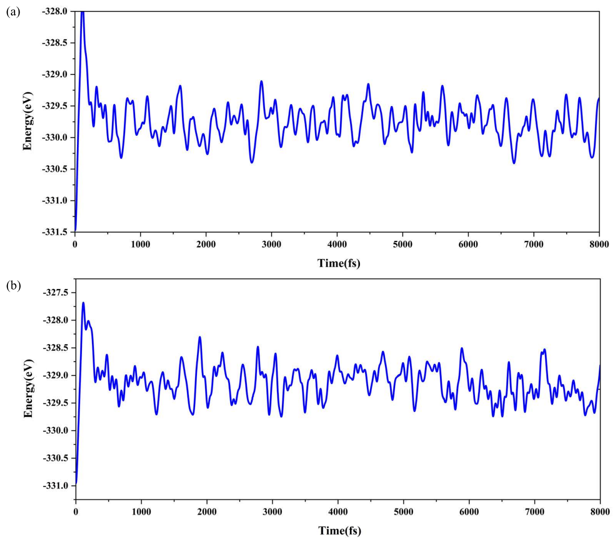


FIG. S6. The total potential energy fluctuation by using ab initio MD simulation for bulk $ZrTe_4Se$ under (a) 3 % uniaxial strain along the [100] direction and (b) 7 % uniaxial strain along the [111] direction.

Part VIII The evolution lines of Wannier centers for bulk $ZrTe_4Se$ under 3 % uniaxial strain.

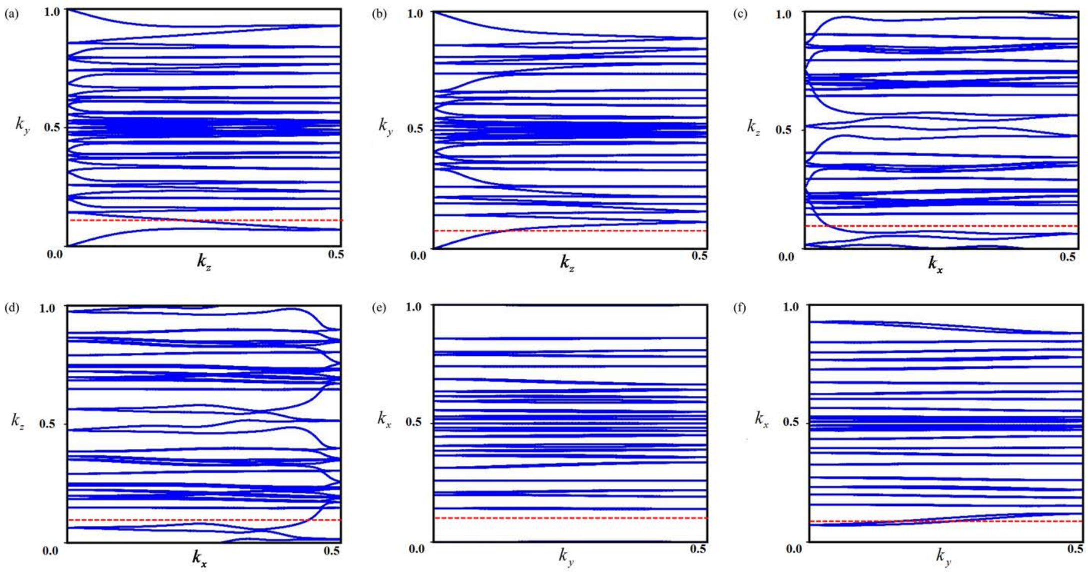


FIG. S7. The evolution lines of Wannier centers for bulk $ZrTe_4Se$ under 3 % uniaxial strain at (a) $k_x$=0.0, (b) $k_x$=0.5, (c) $k_y$=0.0, (d) $k_y$=0.5, (e) $k_z$=0.0 and (f) $k_z$=0.5 planes, respectively. The evolution lines cross the red reference line an odd number of times get the $Z_2$ = 1, otherwise $Z_2$ = 0.

---

* yongliu@ysu.edu.cn,or ycliu@ysu.edu.cn
